# Supplementary material for: Predicting hot-electron free energies from ground-state data
Source: arXiv:2205.05591 ancillary file (2022-09-28)
Supplement: Supplementary file 1 [file Hot_Electrons_Supp_Mat.pdf]

# Predicting hot electrons free energies from ground-state data
## *Supplemental Material*

Chiheb Ben Mahmoud,[1] Federico Grasselli,[1] and Michele Ceriotti[1]

[1]*Laboratory of Computational Science and Modeling, IMX,*
*École Polytechnique Fédérale de Lausanne, 1015 Lausanne, Switzerland*

(Dated: September 28, 2022)

## S1. FULL DERIVATION OF EQ. (5) OF THE MANUSCRIPT

In this Section we prove that the change in the total internal energy, due to a change $\Delta f_i$ in the occupations of the levels, is given by Eq. (5) of the main text:

$$\Delta E \equiv \Delta(E_{\rm b} - E_{\rm dc} + E_{\rm ion}) \approx \sum_i \epsilon_i^0 \, \Delta f_i, \tag{S1}$$

where $\epsilon_i^0$ are the unperturbed Kohn-Sham eigenvalues, computed at a reference electronic temperature, e.g. $T = 0$. The Coulomb interaction between ionic (pseudo)cores does not depend on $f_i$, so $\Delta E_{\rm ion} = 0$. We start with the variation of the band energy due to a change in the occupation of the $j$-th level:

$$\frac{\delta E_{\rm b}}{\delta f_j} = \epsilon_j + \sum_i f_i \frac{\delta \epsilon_i}{\delta f_j} \tag{S2}$$

In first-order perturbation theory, we have (indicating with the superscript "0" the unperturbed quantities)

$$\left.\frac{\partial \rho(\mathbf{r})}{\partial f_j}\right|_{\Delta \mathbf{f}=0} = |\phi_j^0(\mathbf{r})|^2 =: \rho_j^0(\mathbf{r}), \tag{S3}$$

with no change on the eigenfunctions due to further self-consistent cycles. The eigenenergy of the $i$-th KS state is

$$\epsilon_i = \langle \phi_i | \hat{T} + \hat{V}_{\rm ion} + \hat{V}_{\rm scf} | \phi_i \rangle, \tag{S4}$$

where $\hat{V}_{\rm ion}$ is the ion potential and

$$V_{\rm scf}(\mathbf{r}) = \int \frac{\rho(\mathbf{r}')}{|\mathbf{r} - \mathbf{r}'|} d\mathbf{r}' + V_{\rm xc}[\rho](\mathbf{r}) \tag{S5}$$

Therefore, the variation of $\epsilon_i$ under a change in the occupation of the $j$-th KS state is

$$\frac{\delta \epsilon_i}{\delta f_j} = \langle \phi_i | \frac{\delta \hat{V}_{\rm scf}}{\delta f_j} | \phi_i \rangle = \iint \rho_i^0(\mathbf{r}) \left( \frac{1}{|\mathbf{r} - \mathbf{r}'|} + \frac{\delta V_{\rm xc}[\rho]}{\delta \rho(\mathbf{r}')} \right) \rho_j^0(\mathbf{r}') d\mathbf{r}' d\mathbf{r} \tag{S6}$$

since both $\frac{\delta \hat{V}_{\rm ion}}{\delta f_j}$ and $\frac{\delta \hat{T}}{\delta f_j}$ vanish [1], and

$$\frac{\delta V_{\rm scf}(\mathbf{r})}{\delta f_j} = \int \frac{\rho_j^0(\mathbf{r}') d\mathbf{r}'}{|\mathbf{r} - \mathbf{r}'|} + \int \frac{\delta V_{\rm xc}[\rho]}{\delta \rho(\mathbf{r}')} \rho_j^0(\mathbf{r}') d\mathbf{r}'. \tag{S7}$$

In conclusion, the variation of the band energy due to a change in $f_j$ is

$$\frac{\delta E^{\rm b}}{\delta f_j} = \epsilon_j + \sum_i f_i \left[ \iint \frac{\rho_i^0(\mathbf{r}') \rho_j^0(\mathbf{r})}{|\mathbf{r} - \mathbf{r}'|} d\mathbf{r} d\mathbf{r}' + \iint \frac{\delta V_{\rm xc}}{\delta \rho(\mathbf{r}')} \rho_i^0(\mathbf{r}) \rho_j^0(\mathbf{r}') d\mathbf{r} d\mathbf{r}' \right]. \tag{S8}$$

For the double-counting term, we have

$$-\frac{\delta E_{\rm dc}}{\delta f_j} = -\frac{\delta E_{\rm H}}{\delta f_j} + \int \underbrace{\frac{\delta E_{\rm xc}}{\delta \rho(\mathbf{r})}}_{V_{\rm xc}[\rho](\mathbf{r})} \underbrace{\frac{\partial \rho(\mathbf{r})}{\partial f_j}}_{\rho_j^0(\mathbf{r})} d\mathbf{r} - \frac{\delta}{\delta f_j} \int V_{\rm xc}[\rho](\mathbf{r}) \sum_i f_i \rho_i^0(\mathbf{r}) d\mathbf{r} \tag{S9}$$

where

$$E_{\rm H} = \frac{1}{2} \iint \frac{\rho(\mathbf{r}') \rho(\mathbf{r})}{|\mathbf{r} - \mathbf{r}'|} d\mathbf{r} d\mathbf{r}' \tag{S10}$$

---

[1] The first step in Eq. (S6) is justified by the Hellmann-Feynman theorem even without the approximation of Eq. (S3). The ZTA enters Eq. S6, where we neglect the *explicit* dependency of $V_{\rm xc}$ upon the electronic temperature.

is the Hartree energy. Therefore,

$$-\frac{\delta E_{\rm H}}{\delta f_j} = -\frac{\partial}{\partial f_j}\frac{1}{2}\sum_i\sum_l f_i f_l \iint \frac{\rho_i^0(\mathbf{r}')\rho_l^0(\mathbf{r})}{|\mathbf{r}-\mathbf{r}'|}d\mathbf{r}d\mathbf{r}' = -\sum_i f_i \iint \frac{\rho_i^0(\mathbf{r}')\rho_j^0(\mathbf{r})}{|\mathbf{r}-\mathbf{r}'|}d\mathbf{r}d\mathbf{r}', \tag{S11}$$

while

$$-\frac{\partial}{\partial f_j}\int V_{\rm xc}[\rho](\mathbf{r})\sum_i f_i\rho_i^0(\mathbf{r})d\mathbf{r} = -\int V_{\rm xc}[\rho](\mathbf{r})\rho_j^0(\mathbf{r})d\mathbf{r} - \iint \frac{\delta V_{\rm xc}[\rho]}{\delta\rho(\mathbf{r}')}\underbrace{\frac{\partial\rho(\mathbf{r}')}{\partial f_j}}_{\rho_j^0(\mathbf{r}')}\sum_i f_i\rho_i^0(\mathbf{r})d\mathbf{r}'d\mathbf{r}. \tag{S12}$$

Therefore, the first-order derivative of the double-counting term is

$$-\frac{\delta E_{\rm dc}}{\delta f_j} = -\sum_i f_i\left[\iint \frac{\rho_i^0(\mathbf{r}')\rho_j^0(\mathbf{r})}{|\mathbf{r}-\mathbf{r}'|}d\mathbf{r}d\mathbf{r}' + \iint \frac{\delta V_{\rm xc}[\rho]}{\delta\rho(\mathbf{r}')}\rho_i^0(\mathbf{r})\rho_j^0(\mathbf{r}')d\mathbf{r}d\mathbf{r}'\right], \tag{S13}$$

which exactly cancels $\sum_i f_i\frac{\delta\epsilon_i}{\delta f_j}$ when Eq. (S6) is used, thus proving Eq. (5) in the main text. This derivation is based on variations of $f_i$ with respect to given reference values, which need not be necessarily those at $T=0$, which provides a way to further extend the range of applicability of the approximation at very high $T^{\rm el}$ by computing data at a few self-consistent reference temperatures.

## S2. ELECTRONIC ENTROPY

When we are interested in the free energy, we may ask whether to use zero-$T^{\rm el}$ or finite-$T^{\rm el}$ values in the formula for the entropy. Notice that, since energy eigenstates do not enter directly (but only through the occupations), the order is higher than in the case of the internal energy. What we aim at is a good approximation of a possible correction

$$-T\delta^T S \equiv -T[S^T(T) - S^0(T)] \tag{S14}$$

where

$$S^\tau(T) \equiv -k_B\sum_i f_i^\tau(T)\ln[f_i^\tau(T)] + [1-f_i^\tau(T)]\ln[1-f_i^\tau(T)] \tag{S15}$$

and

$$f_i^\tau(T) \equiv f\left(\frac{\epsilon_i^\tau - \mu^\tau(T)}{k_B T}\right) \tag{S16}$$

Here $\epsilon_i^\tau$ is the $i$-th eigenenergy computed at temperature $\tau$, while $\mu^\tau(T)$ is the chemical potential obtained from the normalisation relation, when the employed states are $\epsilon_i^\tau$ but the temperature use to populate the states is $T$. The symbol $\delta^\tau$ denotes a change, at fixed population temperature $T$, due to a variation $\tau$ of the temperature used in the calculation of the eigenstates:

$$\delta^\tau f_i(T) \equiv f\left(\frac{\epsilon_i^\tau - \mu^\tau(T)}{k_B T}\right) - f\left(\frac{\epsilon_i^0 - \mu^0(T)}{k_B T}\right) \tag{S17}$$

At first order in $\delta^\tau f(T)$ we obtain

$$\begin{aligned} -T\delta^\tau S &\approx -T\sum_i \left.\frac{\partial S}{\partial f_i}\right|_{f_i^0(T)}\delta^\tau f_i(T) \\ &= -k_B T\sum_i \ln\left(\frac{1-f_i^0(T)}{f_i^0(T)}\right)\delta^\tau f_i(T) \\ &= -\sum_i(\epsilon_i^0 - \mu^0(T))\delta^\tau f_i(T) \end{aligned} \tag{S18}$$

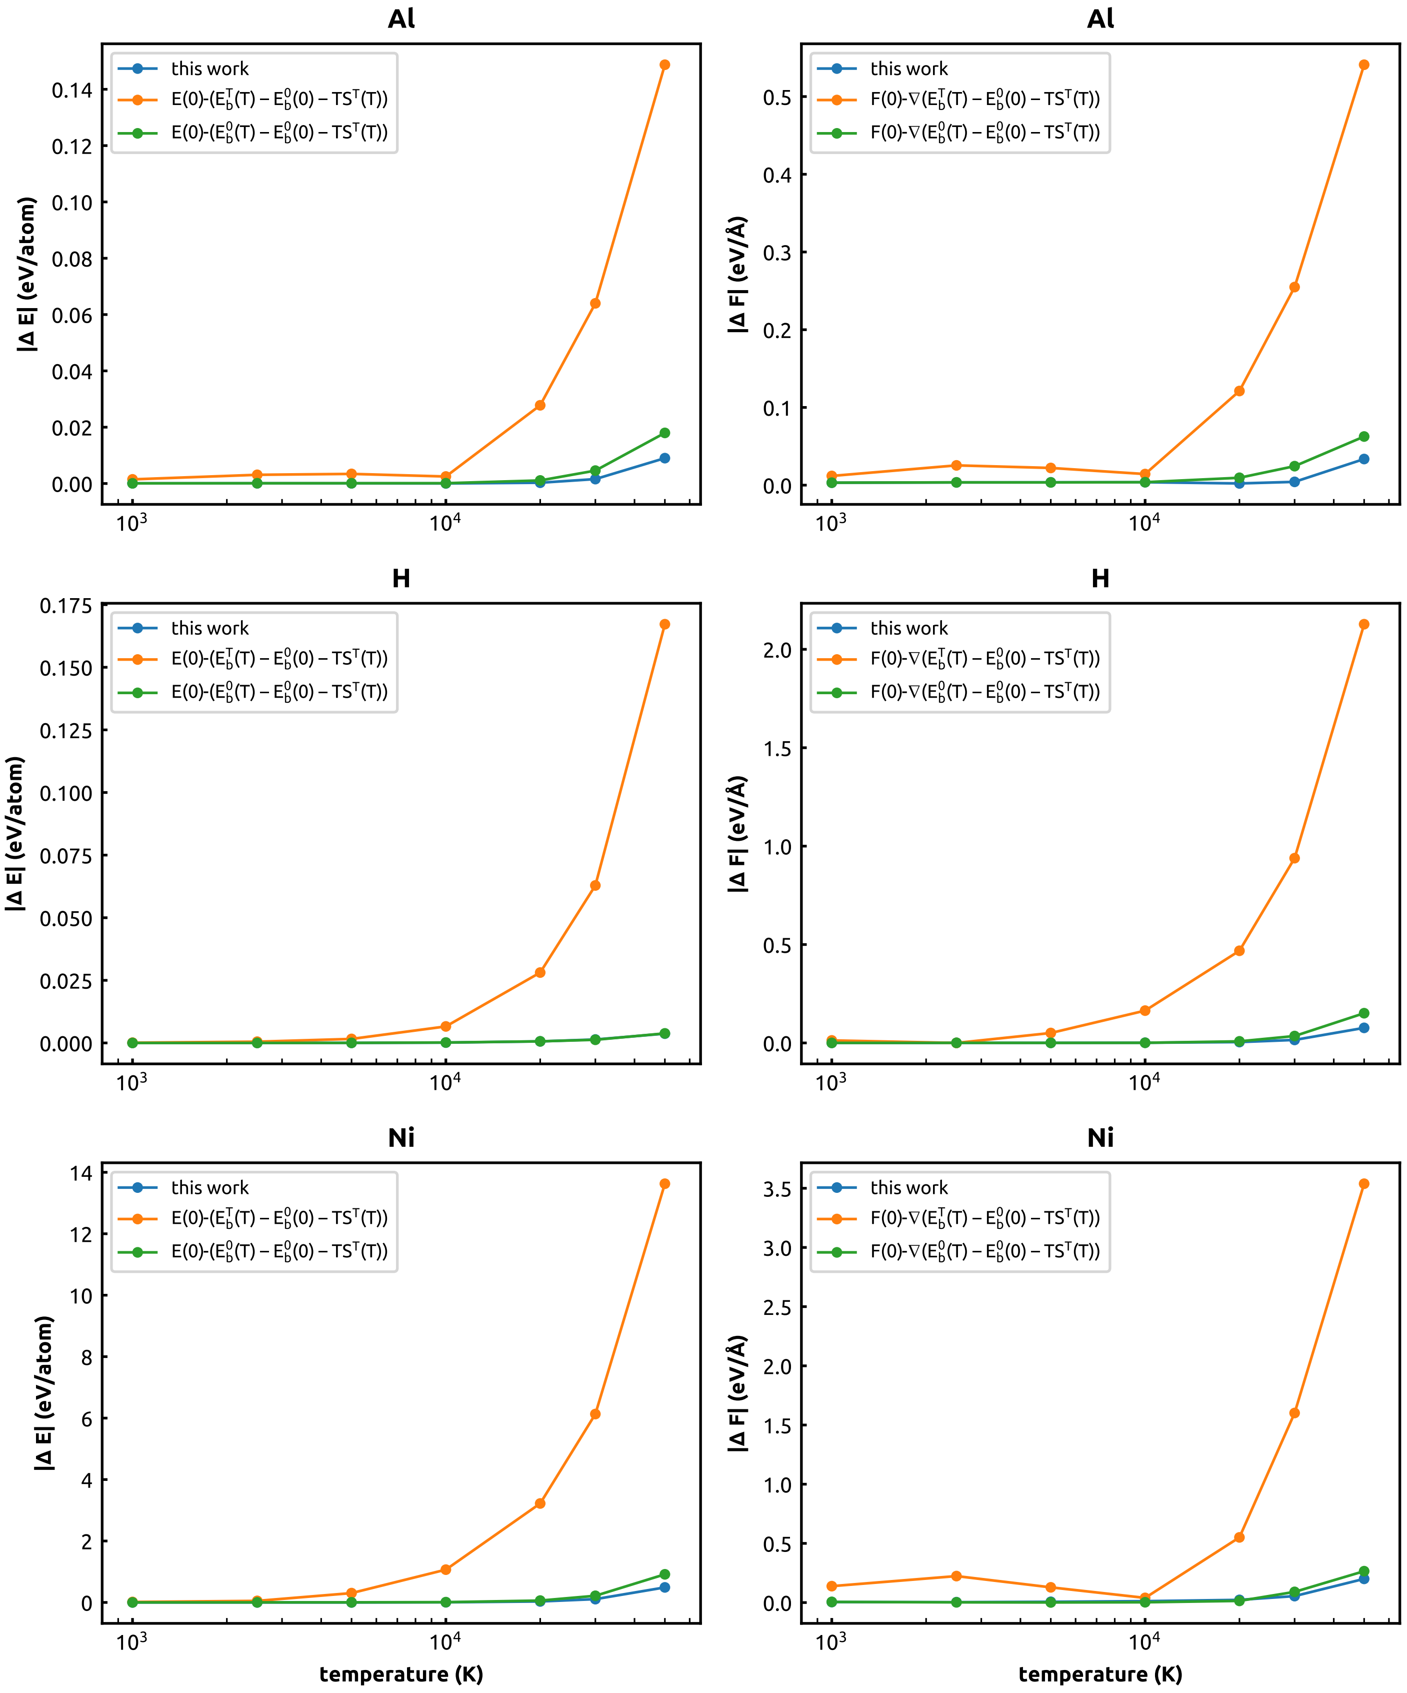


Figure S1: Errors, with respect to the finite-$T^{\mathrm{el}}$ results, of different methods to compute a finite-$T^{\mathrm{el}}$ correction to the total energy and the atomic force, computed for a single force component in an aluminum supercell, a liquid hydrogen structure and a liquid nickel structure as a function of the electronic temperature.

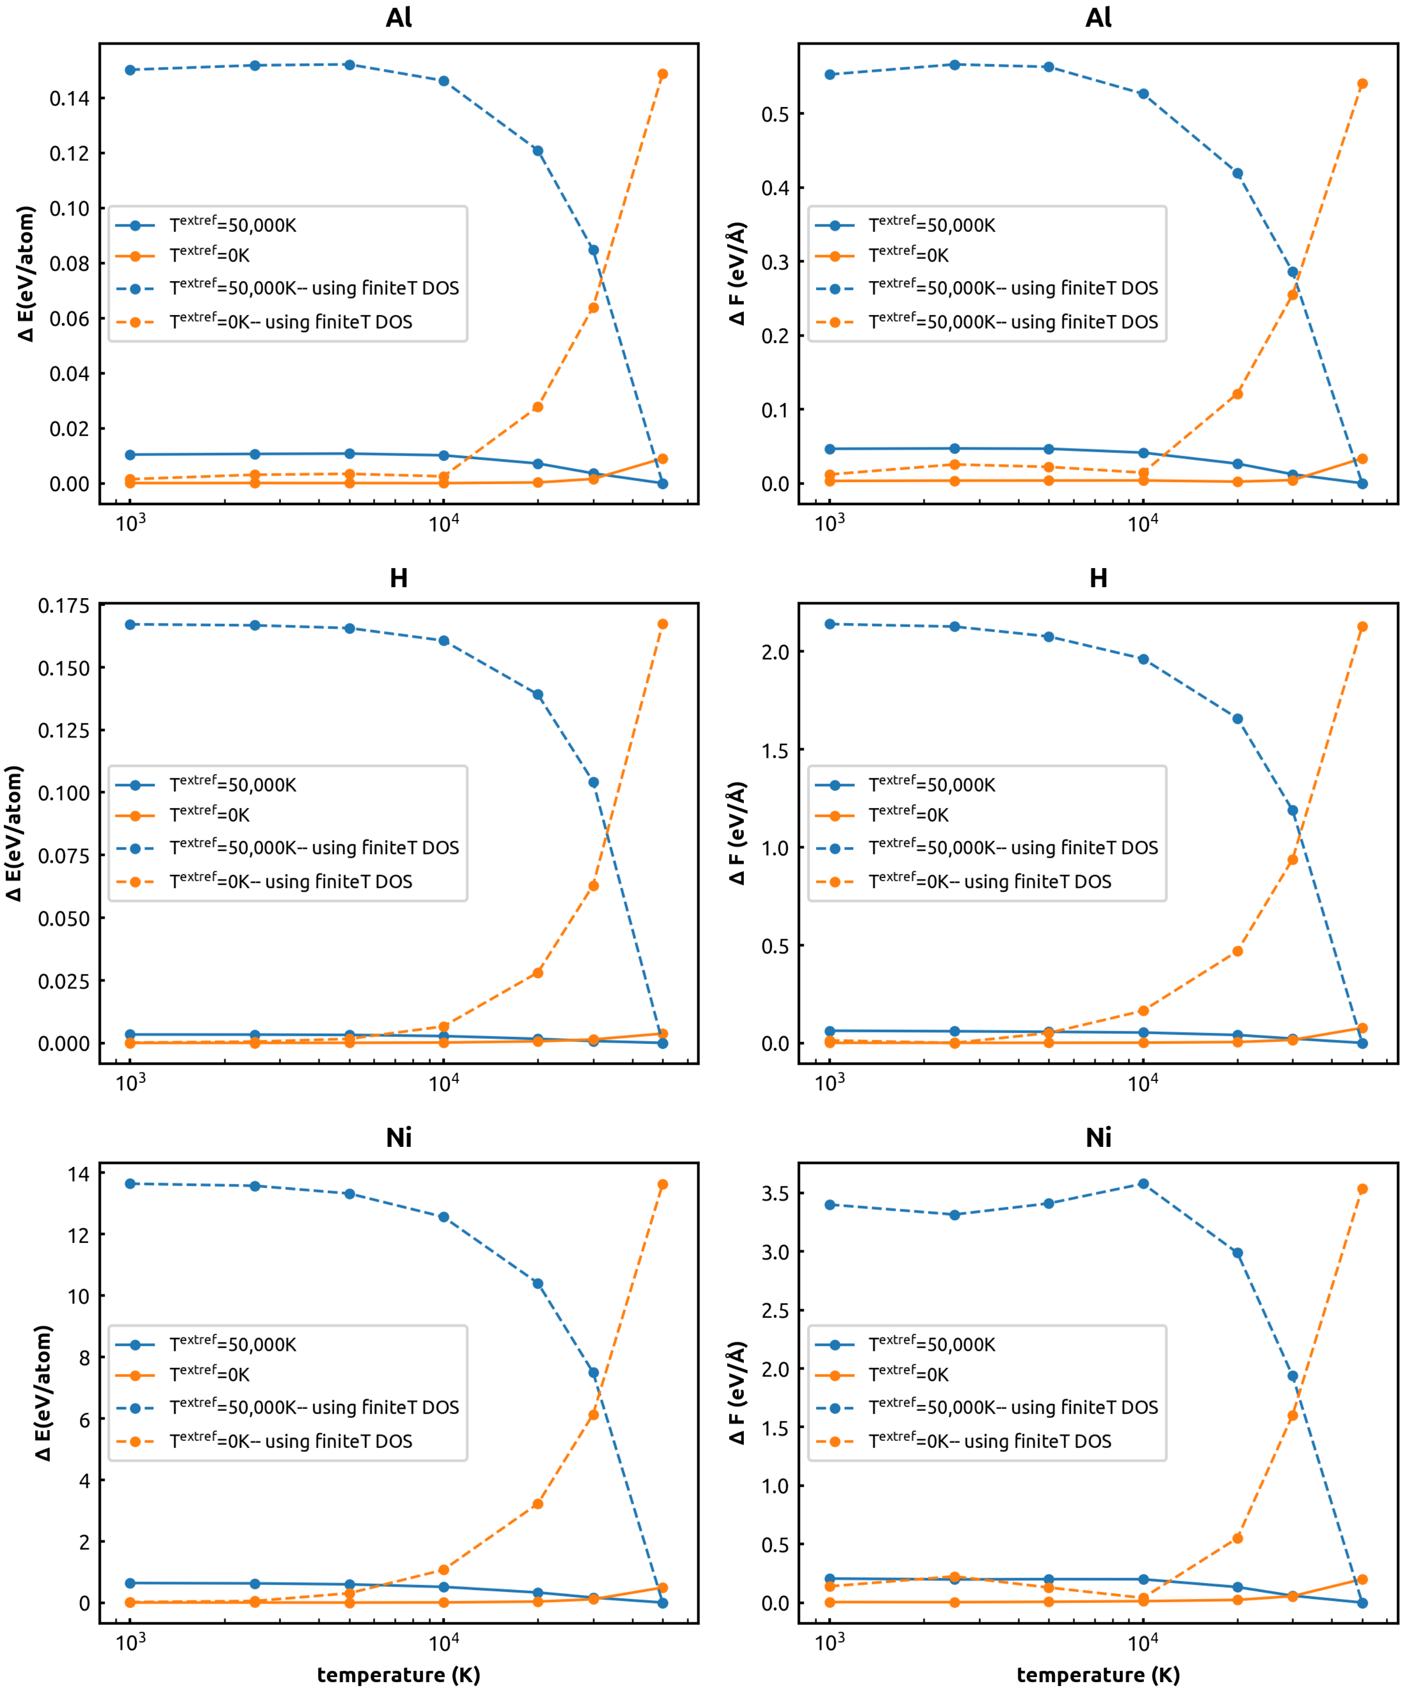


Figure S2: Errors, with respect to the finite-$T^{\mathrm{el}}$ results, of different methods to compute a finite-$T^{\mathrm{el}}$ and using two reference calculations done at $T^{\mathrm{el}} = 50,000$K and $T^{\mathrm{el}} = 0$K, to compute a correction to the total energy and the atomic force, computed for a single force component in an aluminum supercell, a liquid hydrogen structure and a liquid nickel structure as a function of the electronic temperature.

Taking $\tau = T$, the term $-\sum_i \epsilon_i^0[f_i^T(T) - f_i^0(T)]$ *cancels* with an analogous term arising in $\Delta E$, as it is evident when we add and subtract $f_i^0(T)$ in $\Delta f_i = f_i^T(T) - f_i^0(0)$ used in Eq. (S1), while $\sum_i \mu^0(T)\delta^\tau f_i(T) = 0$ because the total number of electrons is fixed.

In conclusion, the formula to use for the Helmholtz free energy -corrected up to a change in both the population and the finite temperature energies appearing in the total energy and the entropic contribution- is:

$$A(T) \approx A^0(T) \equiv E(0) + \sum_i \epsilon_i^0[f_i^0(T) - f_i^0(0)] - TS^0(T) \tag{S19}$$

that is, where only the zero-$T$ levels, i.e. the zero-$T$ DOS, are considered all along. As discussed in more details in Sec. S7, this quantity is defined up to an energy alignment constant which disappears when gradients are computed. Figure S1 shows the different ways one can use to incorporate the finite-$T^{\rm el}$ correction to the atomic force, computed for a single atomic force in an aluminum supercell.Figure S2 shows, in particular, the use of the DOS computed at $T^{\rm el} = 50,000$K and trying to recover the free energy and force of lower temperature calculations compared to the finite temperature DFT. The relative errors are larger at low temperatures, which indicates that the approximation of this work is better used when the reference calculation is done at low temperature. This behaviour occurs despite a minimal change in the DFT DOS computed at $T^{\rm el} = 0$K and $T^{\rm el} = 50,000$K. In Fig. S3 shows the DOS of a liquid hydrogen structure computed at the mentioned temperatures. We also remark that the conditions considered in Figs. S1 and S2 are consistent with WDM conditions as reported in the literature [1, 2].

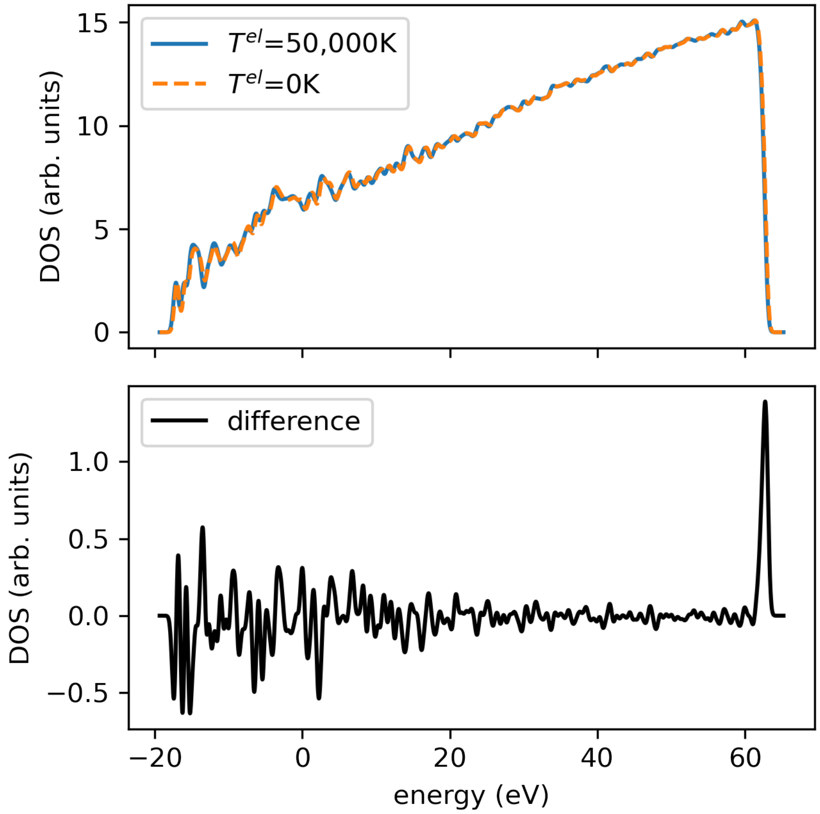


Figure S3: (Upper panel) The DOS of a liquid hydrogen structure using two electronic temperatures. Blue: ground-state, orange: $T^{\rm el}$=50,000K. The Gaussian broadening used to construct the DOS is 0.3eV. (Lower panel) The residual between the two DOS computed at $T^{\rm el} = 0$K and $T^{\rm el} = 50,000$K.

## S3. FORCE FITTING FROM FINITE-T DATA

In this section we discuss the different ways one can fit the interatomic force from finite-$T^{\mathrm{el}}$ data. We consider five different cases for a single force component of a liquid hydrogen snapshot, which is the same one used to illustrate the approximation developed in this work in Figs. S1 and S2:

- the force extrapolation from this work's approximation, with reference calculation done at the ground-state $T_0 = 0$K, $F^{T_0 \to T_{\max}}(T^{\mathrm{el}})$
- the force extrapolation from this work's approximation, with reference calculation done at $T_{\max} = 50,000$K, $F^{T_{\max} \to T_0}(T^{\mathrm{el}})$
- a linear fit between the ground-state force and the finite-$T^{\mathrm{el}}$ force computed at $T^{\mathrm{el}} = 50,000$K
- a linear combination of the previous two predictions in a way to approximate the finite-$T^{\mathrm{el}}$ force with the better approximation according to the following mixing:

$$F^{\mathrm{two-point}}(T^{\mathrm{el}}) = \frac{T^{\mathrm{el}} - T_0}{T_{\max} - T_0} F^{T_0 \to T_{\max}}(T^{\mathrm{el}}) + \frac{T_{\max} - T^{\mathrm{el}}}{T_{\max} - T_0} F^{T_{\max} \to T_0}(T^{\mathrm{el}}),$$

- a cubic fitting using the two previous predictions $F^{T_0 \to T_{\max}}(T^{\mathrm{el}})$ and $F^{T_{\max} \to T_0}(T^{\mathrm{el}})$ using our approximation

$$F^{\mathrm{two-point,cubic}}(T^{\mathrm{el}}) = \left[1 - \lambda\left(\frac{T^{\mathrm{el}} - T_0}{T_{\max} - T_0}\right)\right] F^{T_0 \to T_{\max}}(T^{\mathrm{el}}) + \lambda\left(\frac{T^{\mathrm{el}} - T_0}{T_{\max} - T_0}\right) F^{T_{\max} \to T_0}(T^{\mathrm{el}}),$$

  where $\lambda(x)$ is the cubic polynomial that satisfies $\lambda(0) = 0$, $\lambda(1) = 1$, $\lambda'(0) = \lambda'(1) = 0$

We report our findings about the errors of these methods compared to finite-$T^{\mathrm{el}}$ computed forces in Fig. S4. The simple linear fit yields worse results than all the other methods, except at the extremes (0K and 50,000K). Our Mermin-like functional used as a single-point extrapolation seems to be a good approximation on its own when using a round-state reference, while the high-$T$ reference leads to high errors at low temperature. A linear mixing of the high and low-temperature extrapolations improves the accuracy in the high-temperature limit, and can be further improved by considering that in our Mermin-functional expansion the error has zero first derivative close to the edges, and that this property can be preserved by using a mixing function that has zero derivatives at the edges.

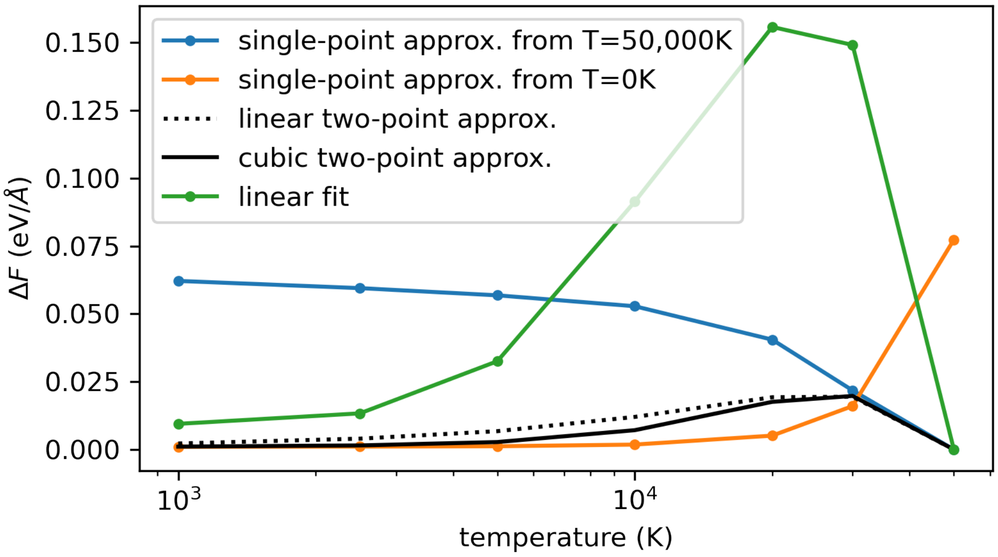


Figure S4: Calculation errors compared to the finite-$T^{\mathrm{el}}$ force in a liquid hydrogen structure.

## S4. FORCES DUE TO HOT ELECTRONS

Here we show the derivation of the formula for the temperature-dependent part of the total forces due to the presence of hot electrons:

$$\Delta\mathbf{F}_I(T) = -\nabla_I \Delta A(T), \tag{S20}$$

where $\Delta A(T) = \Delta E_b^0(T) - TS^0(T)$ is the free energy of the hot electrons. The band energy term $\Delta E_b^0(T)$ is defined as the difference between the band energies of electron system at $T = 0$ and $T > 0$:

$$\Delta E_b^0(T) = \int_{-\infty}^{+\infty} \mathrm{d}\epsilon\ \epsilon g^0(\epsilon)[f(\frac{\epsilon-\mu(T)}{k_B T}) - f(\frac{\epsilon-\mu(0)}{k_B 0^+})], \tag{S21}$$

where $f(\frac{\epsilon-\mu(T)}{k_B T}) = 1/(1+exp(-(\epsilon-\mu(T))/(k_B T))$ is the Fermi-Dirac occupation at a temperature $T$ and $\mu(T)$ is the Fermi level at a temperature $T$ derived from the charge neutrality of the electron system of size $N$:

$$N = \int_{-\infty}^{+\infty} \mathrm{d}\epsilon\ g^0(\epsilon) f(\frac{\epsilon-\mu(T)}{k_B T}). \tag{S22}$$

The entropy is defined canonically as:

$$S_{KS}(T) \ = \ -k_B \int_{-\infty}^{+\infty} \mathrm{d}\epsilon\ \ g^0(\epsilon)[f(\frac{\epsilon-\mu(T)}{k_B T})\log(f(\frac{\epsilon-\mu(T)}{k_B T})) + (1 - f(\frac{\epsilon-\mu(T)}{k_B T}))\log(1 - f(\frac{\epsilon-\mu(T)}{k_B T}))]. \tag{S23}$$

From these equations, we notice that taking the gradient of these components requires the determination of the gradient of the Fermi level $\mu(T)$ with respect to the atomic positions because of the chain rule. One easy way to determine this gradient is by taking the derivative of Eq. S22 at fixed total number of electrons is unaffected by perturbing the system and we obtain:

$$\nabla_I \mu(T) = -\frac{1}{\int \mathrm{d}\epsilon\ g^0(\epsilon)\frac{\partial f}{\partial \mu}} \int_{-\infty}^{+\infty} \mathrm{d}\epsilon\ f(\frac{\epsilon-\mu(T)}{k_B T})\nabla_I g^0(\epsilon). \tag{S24}$$

In the limit of $T = 0$, the Fermi level becomes the Fermi energy $\mu(0) = \epsilon_F$ and we obtain:

$$\nabla_I \epsilon_F = -\frac{1}{g^0(\epsilon_F)} \int_{-\infty}^{\epsilon_F} \mathrm{d}\epsilon\ \nabla_I g^0(\epsilon).$$

The thermal band energy of Eq. S21 is the difference between two similar terms, that is why we only focus on the first term depending on $T > 0$, $E_b(T)$, since it is the general case of the $T = 0$ term. In order to make notations easier to follow, we write $f = f(\frac{\epsilon-\mu(T)}{k_B T})$. We start by writing the gradient of $E_b(T)$:

$$\nabla_I E_b(T) = \int \mathrm{d}\epsilon\ \epsilon f \nabla_I g^0(\epsilon) + \int \mathrm{d}\epsilon\ \epsilon g^0(\epsilon)\frac{\partial f}{\partial \mu}\nabla_I \mu. \tag{S25}$$

By plugging Eq. S24 in the previous equation and rearranging terms, we obtain the following expression for the gradients of the band energy as a function of the gradient of the electronic density of states:

$$\nabla_I E_b(T) = \int \mathrm{d}\epsilon\ (\epsilon - \Sigma) f \nabla_I g^0(\epsilon), \tag{S26}$$

where $\Sigma = \frac{\int \mathrm{d}\epsilon\ \epsilon g^0(\epsilon)\frac{\partial f}{\partial \mu}}{\int \mathrm{d}\epsilon\ g^0(\epsilon)\frac{\partial f}{\partial \mu}}$ is an average shift term appearing due to the conservation of the Fermi level. In the $T = 0$ limit, this shift is the Fermi energy of the electron system: $\Sigma(T = 0) = \epsilon_F$.

We follow the same logic in determining the gradient of the entropy $S^0(T)$:

$$\nabla_I S^0(T) = -k_B \int \mathrm{d}\epsilon\ [f\log(f) + (1-f)\log(1-f)]\nabla_I g^0(\epsilon) - k_B \int \mathrm{d}\epsilon\ \frac{\partial[f\log(f) + (1-f)\log(1-f)]}{\partial \mu}\nabla_I \mu. \tag{S27}$$

In this expression, we need to simplify the derivative with respect to $\mu$ in the second integral and we obtain:

$$\frac{\partial[f\log(f) + (1-f)\log(1-f)]}{\partial \mu} = \log(\frac{f}{1-f})\frac{\partial f}{\partial \mu} = -\beta(\epsilon - \mu)\frac{\partial f}{\partial \mu}. \tag{S28}$$

We plug this expression along side Eq.S24 in Eq. S27, rearrange terms and obtain the following expression for the gradient of the entropy:

$$\nabla_I S^0(T) = -k_B \int \mathrm{d}\epsilon \ [f\log(f) + (1 - f)\log(1 - f)]\nabla_I g^0(\epsilon) + \frac{1}{T}(\mu - \Sigma) \int \mathrm{d}\epsilon \ f\nabla_I g^0(\epsilon), \quad \text{(S29)}$$

where we notice that the shift term $\Sigma$ appears again acting on the Fermi level of the electron system. This derivation proves that we can write the hot electron forces just in terms of the gradients of the DOS, which can be computed easily within our ML approach. The advantage of this derivation is that it can be extended to the case of the gradients of $F^{el}(T)$ with respect to the cell vectors in order to obtain the stress virial. Only the gradients of the DOS with respect to the atomic positions need to be replaced by the gradients of the DOS with respect to the variations of the cell vectors.

## S5. DETAILS ABOUT THE DFT CALCULATIONS

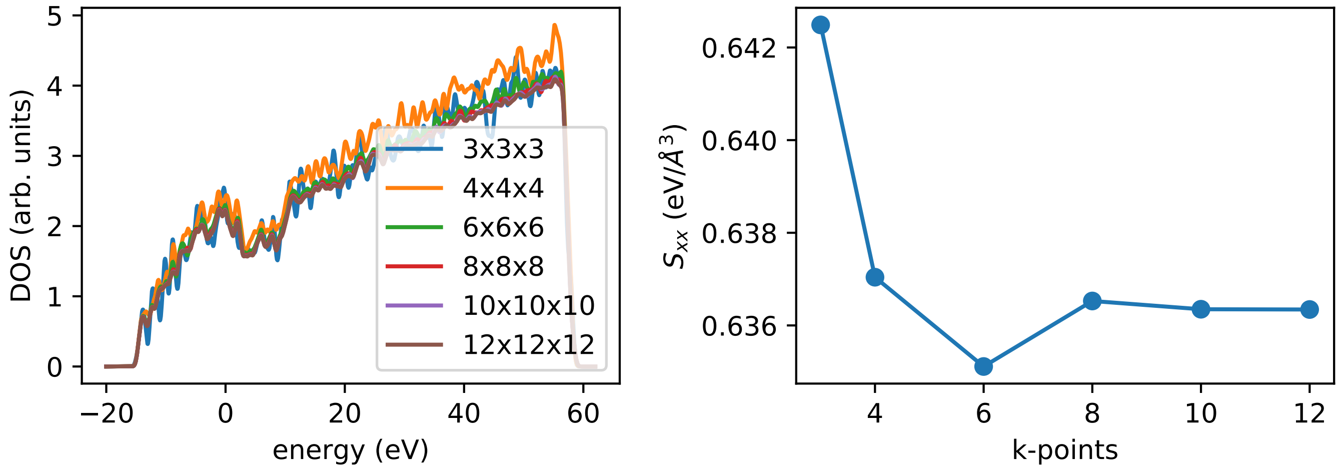


Figure S5: Convergence of some key quantities with respect to the k point grid for a 64-atom liquid hydrogen structure. Left: electronic density of states constructed using a Gaussian broadening value of 0.3eV. Right: the $S_{xx}$ component of the Hellmann-Feynman stress tensor. In both cases $8 \times 8 \times 8$ corresponds to the targeted k-point spacing of 0.01Å$^{-1}$.

We use QUANTUM ESPRESSO [3–5] to perform the density functional theory (DFT) calculations of the metallic hydrogen training set using the DF2 van der Waals density functional [6–9] and the Optimized Norm Conserving Vanderbilt (ONCV) pseudopotential [10]. We use a plane-wave energy cutoff on wave functions of 100Ry. We use the Marzari-Vanderbilt cold smearing [11] of 0.01Ry which yielded similar energies and forces to calculations done at higher k-point density and with a Fermi-Dirac smearing of 10K. The self-consistency accuracy in the electron density is $1 \times 10^{-12}$Ry. We use dense k-point mesh targeting at least 0.01Å$^{-1}$ spacing to ensure the convergence of the DOS and the stress tensor. We perform these convergence test on a hydrogen structure containing 64 atoms and of density 0.733g cm$^{-3}$. The results of the convergence tests with respect to the k-point grid for the DOS (to the left) and the $S_{xx}$ component of the stress tensor (to the right) are shown in Figure S5. In our calculations we make sure to compute a sufficient number of bands to accommodate the tail of the distribution, which reaches high energies at large $T^{\mathrm{el}}$. In practice, we choose to compute 3 bands per atom, which results in the computation of 6 electronic states per atom. This choice ensures that the Fermi-Dirac occupation of the highest energy level is below $1 \times 10^{-5}$ when $T^{\mathrm{el}} = 50,000$K. We find that this value is sufficiently low to not affect the values of the atomic forces.

We also use QUANTUM ESPRESSO to perform the DFT calculations for the tests on the aluminum and nickel systems. For the former we use a wavefunction energy cutoff of 45Ry, Marzari-Vanderbilt smearing, PBE[12] exchange-correlation functional and a k-point mesh of 12×12×12, and for the latter we use the same parameters except for the wavefunction energy cutoff of 60Ry and a k-point density mesh of 10×10×10.

## S6. DETAILS ABOUT THE ML MODELS

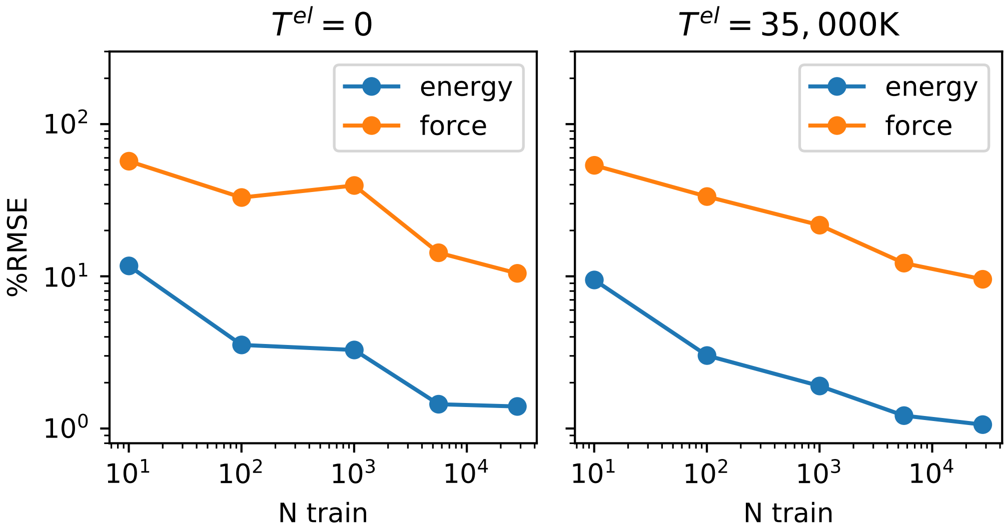


Figure S6: Root mean square error (RMSE) as a percentage of the total variance of the energies and forces as a function of the size of the training set. Left: from the GAP model; right: from the GAP and the finite-$T^{\mathrm{el}}$ correction at $T^{\mathrm{el}} = 35,000$K.

We train a GAP model, to learn and predict the $T^{\mathrm{el}} = 0$ contribution to the total free energy, on the total DFT energies and a single Hellmann-Feynman force component per structure. We decompose the total energy into a 2-body term a many-body:

$$E = E_{2B} + E_{MB}. \tag{S30}$$

The 2-body term $E_{2B}$ is fitted on dissociating hydrogen dimers placed in large box of length 15Å. The distances range from 0.075Å to 0.73Å, which corresponds to the repulsive part of the pair interaction. This 2-body term ensures the stability of our molecular dynamics simulations at high temperatures (>20,000K). In practice, we tabulate these values and use LAMMPS[13] to handle the calculations of the atomic energies and forces of the 2-body interactions. The many-body term is obtained from the Smooth Overlap of Atomic Positions (SOAP) [14, 15] representation with radial scaling [16]. The SOAP representation requires the optimization of several hyperparameters, that we achieve using a grid-search. We select the parameters that minimize the prediction error on the total energy in a subset of 5000 structures using a 2-fold cross-validation regression scheme. The best SOAP parameters are (in the notation of *librascal* [17]): *max_radial*=8, *max_angular*=6, *interaction_cutoff*=2Å, *gaussian_sigma_constant*=0.1 and the best radial scaling parameters are: *rate*=1.0, *scale*=2.0 and *exponent*=4.

We follow a similar approach to the many-body term to construct an atom-centered model for the electronic density of states (DOS) [18]. We build the DOS from the KS eigenenergies of the same calculations for the total energies using a Gaussian broadening of 0.5eV. We also build a single DOS-gradient component, computed by finite displacement of a single atom by $1 \times 10^{-3}$Å.

The model also relies on the SOAP representation. We use a grid-search on the same subset to find the optimal hyperparameters that minimize the prediction errors on the DOS: *max_radial*=12, *max_angular*=8, *interaction_cutoff*=4Å, *gaussian_sigma_constant*=0.1 and the best radial scaling parameters are: *rate*=1.0, *scale*=1.0 and *exponent*=2.

We use the Projected process approximation of the Gaussian process regression framework to train the two ML models. The idea is to select a subselection of the training environments and use them a basis to expand the target quantities (energy or DOS). We select 7000 environments for the GAP model and 5000 environments for the DOS model. These environments are chosen by a greedy algorithm, the furthest point sampling [19]. We validate our two ML models on a validation set containing 2500 structures. Figure S6 shows the learning curves (LCs) of the energies and forces obtained from the GAP model (left) and the full framework, i.e. GAP and the thermal electronic correction (right) at $T^{\mathrm{el}} = 35,000$K. The LCs are still linear for all the considered quantities in the log-log plots and suggest that the accuracy of the models can be enhanced by training on more configurations.

## S7. DETAILS ABOUT THE ELECTRONIC DENSITY OF STATES

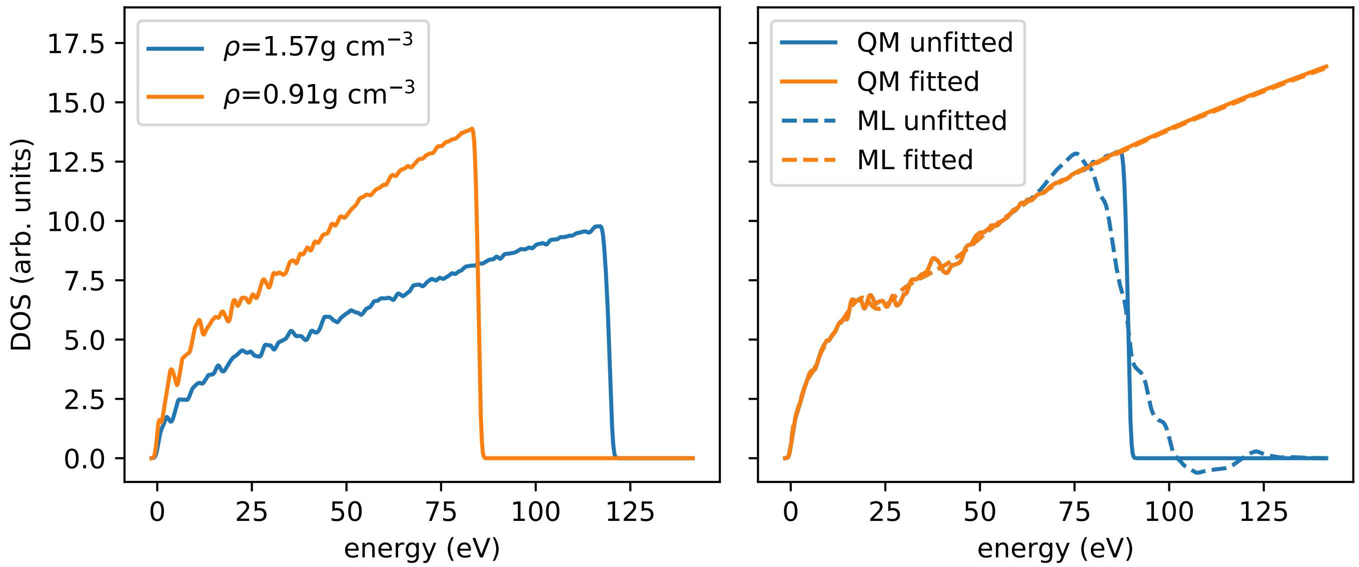


Figure S7: Left: Example of the unfitted DFT DOS of two hydrogen structures at different densities computed using 3 bands per atom. Blue: density is 1.57g cm$^{-3}$; orange: density is 0.91g cm$^{-3}$. Right: A parity plot of the finite-$T^{\mathrm{el}}$ correction computed from unfitted and fitted high energy states of the DFT DOS.

In this paragraph we address a few difficulties when preparing the ML models for the DOS. The alignment of the energy bands is in principle irrelevant to the definition of the finite-$T^{\mathrm{el}}$ correction, according to Eq. S21. While the gradients of the DOS with respect to the atomic positions or the cell vectors may depend on the chosen alignment, the finite-$T^{\mathrm{el}}$ correction to the forces and stress involving them do not. We only need to make sure that the alignment is done consistently when computing the energy terms and the DOS gradients. While there are several strategies to align the DOS, like aligning with respect to the deep core levels, the valence band minimum (VBM) or the Fermi energy, the choice of the alignment should only depend on the quality of the ML prediction. In this case, we find that aligning the DOS with respect to the VBM yields the lowest prediction errors because it uniformizes the energy range on which the DOS is defined. This strategy helps creating uniform targets. However, the dataset contains configurations at different volumes and hence their DOS can span a different energy range, even after VBM alignment, for the same number of the calculated electronic states (c.f. left panel of Figure S7). The calculated DOS drops to zero above the highest computed energy level. Even though the chosen number of energy levels is always such that the Fermi-Dirac occupation of the highest level is negligible even at the largest $T^{\mathrm{el}}$ considered, a sudden, unphysical drop in the DOS negatively affects the learning. To solve this issue, we fit the values of the missing (empty) states to a square root behavior to ensure that the targets for our ML DOS model do not involve unphysical discontinuities. The right panel of Figure S7 shows an example of the effect of such discontinuities on the learning of the DOS in a liquid hydrogen structure, and how fitting the missing bands provides much needed stability to the ML DOS model.

We want to stress that these fitted occupations do not contribute to the finite-$T^{\mathrm{el}}$ correction, even at $T^{\mathrm{el}} = 50,000$K, despite the long tail of the Fermi-Dirac distribution at this temperature. The RMSE of the finite-$T^{\mathrm{el}}$ correction to the atomic forces computed with the DFT fitted and unfitted DOS is 0.00037eV/Å and can be neglected.

## S8. DFT VS ML SIMULATION TIMES

In Fig. S8, we report the computation time and scaling of DFT, using a dense k-point mesh and at Γ point, and ML timesteps for metallic liquid hydrogen simulations at different sizes ranging from 32 atoms to 1024 atoms per structure, as well as the cubic trend in the number of atoms in the structures for the dense k-point DFT mesh calculations. The ML approach presents a nearly linear scaling and is several orders of magnitude less expensive than DFT. We perform the DFT calculations using GPU accelerated nodes with a 12-core Intel Xeon running at 2.6GHz and Nvidia Tesla P100. The 512-atom structure requires 3 nodes. The poor behavior for smaller system is due to the high cost

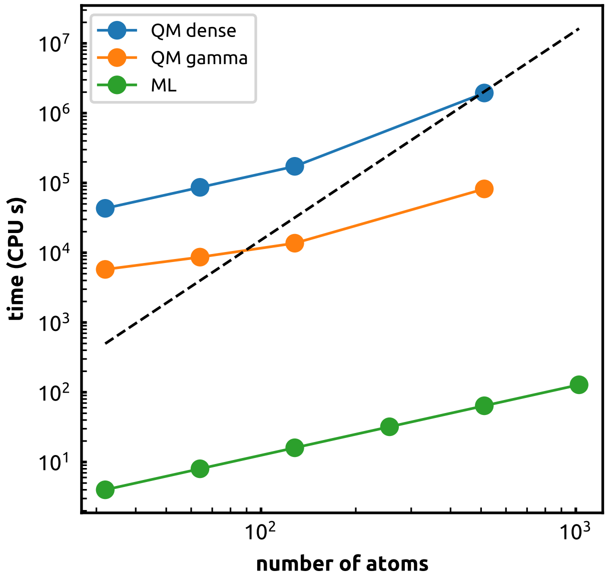


Figure S8: CPU time needed for a single MD timestep for the metallic liquid hydrogen structures of different sizes ranging from 32 atoms to 512 atoms when performing a DFT calculation, with a dense k-point mesh and at Γ point, and from 32 atoms to 1024 atoms when using the ML models, at $T^{\mathrm{el}} = 50,000$K. In the latter case, the time of the SOAP representation is included. The dashed line near the blue curve represents the cubic scaling with the number of atoms in the structure.

of the frequent data transfer between the node's RAM and the GPU VRAM, which offsets the gains from using GPU acceleration. We perform the ML simulations using 4 cores/threads of an Intel Xeon CPU running at 2.6 GHz. For reference, a DFT calculation of 128 atoms can take up to 40GB of RAM, while the ML approach, while it depends on the hyperparameters of the representation, can take up to a few hundreds of MB of RAM for the same configuration.

## S9. CALCULATION OF THE HEAT CAPACITY

To make things simpler we start with the isochoric heat capacity and define the internal energy of the system as

$$U \equiv \frac{3}{2} N_{\mathrm{i}} k_{\mathrm{B}} T + k_{\mathrm{B}} T^2 \left(\frac{\partial \ln Z}{\partial T}\right)_V, \qquad \text{where} \quad Z \equiv \sum_{\mathbf{R}} \exp\left[-\frac{A(\mathbf{R}, T^{\mathrm{el}} = T)}{k_{\mathrm{B}} T}\right]. \tag{S31}$$

In doing this, we have assumed that the configurational partition function of the nuclei is the average, on nuclear configurations $\mathbf{R}$, of the $\mathbf{R}$-dependent canonical partition function, $\exp\left[-\frac{A(\mathbf{R},T^{\mathrm{el}}=T)}{k_{\mathrm{B}}T}\right]$, associated to the electronic problem. The term $\frac{3}{2}N_{\mathrm{i}}k_{\mathrm{B}}T$ accounts for the kinetic energy of the $N_{\mathrm{i}}$ ions. Thus

$$\begin{aligned} U &= \frac{3}{2} N_{\mathrm{i}} k_{\mathrm{B}} T + \frac{1}{Z} \sum_{\mathbf{R}} \left[A(\mathbf{R}, T) - T \left(\frac{\partial A}{\partial T}\right)_V\right] \exp\left[-\frac{A(\mathbf{R}, T)}{k_{\mathrm{B}} T}\right] \\ &= \frac{3}{2} N_{\mathrm{i}} k_{\mathrm{B}} T + \frac{1}{Z} \sum_{\mathbf{R}} E(\mathbf{R}, T^{\mathrm{el}} = T) \exp\left[-\frac{A(\mathbf{R}, T)}{k_{\mathrm{B}} T}\right] \end{aligned} \tag{S32}$$

where we employed the thermodynamic relations

$$E = A + TS \qquad \text{and} \qquad \left(\frac{\partial A}{\partial T}\right)_V = -S. \tag{S33}$$

We remark that here $S = S(\mathbf{R},T)$ is the configuration-dependent electronic entropy. The heat capacity can be thus obtained from finite differences of $U$ in $NVT$ simulations (i.e., where structures are sampled with weight $\frac{1}{Z}\exp\left[-\frac{A(\mathbf{R},T)}{k_\mathrm{B}T}\right]$, since it is the free energy $A(\mathbf{R},T)$ that drives the ionic dynamics):

$$C_V = \frac{U(T+\Delta T)-U(T)}{\Delta T} = \frac{3}{2}N_\mathrm{i}k_\mathrm{B} + \frac{\left\langle E(T^\mathrm{el}=T+\Delta T)\right\rangle_{N,V,T+\Delta T} - \left\langle E(T^\mathrm{el}=T)\right\rangle_{N,V,T}}{\Delta T} \tag{S34}$$

Equivalently, after a lengthy but straightforward calculation–see Eq. (S44) in Sec. S10–, the following fluctuation formula can be derived

$$C_V \equiv \left(\frac{\partial U}{\partial T}\right)_V = \frac{3}{2}N_\mathrm{i}k_\mathrm{B} + \frac{1}{k_BT^2}\left(\langle E\,A\rangle - \langle E\rangle\langle A\rangle\right) - \frac{1}{k_BT}\left(\left\langle E\left(\frac{\partial A}{\partial T}\right)_V\right\rangle - \langle E\rangle\left\langle\left(\frac{\partial A}{\partial T}\right)_V\right\rangle\right) + \left\langle\left(\frac{\partial E}{\partial T}\right)_V\right\rangle. \tag{S35}$$

Notice that, within our approximation, $\left(\frac{\partial E}{\partial T}\right)_V$ reduces to $\left(\frac{\partial E_\mathrm{b}}{\partial T}\right)_V = T\left(\frac{\partial S}{\partial T}\right)_V$. In terms of the free energy driving the dynamics, $A$, and of its derivatives, we can write:

$$\begin{aligned} C_V - \frac{3}{2}N_\mathrm{i}k_\mathrm{B} = {} & \frac{\langle A^2\rangle - \langle A\rangle^2}{k_BT^2} - \frac{2}{k_BT}\left[\left\langle A\left(\frac{\partial A}{\partial T}\right)_V\right\rangle - \langle A\rangle\left\langle\left(\frac{\partial A}{\partial T}\right)_V\right\rangle\right] \\ & + \frac{1}{k_BT}\left[\left\langle\left(\frac{\partial A}{\partial T}\right)_V^2\right\rangle - \left\langle\left(\frac{\partial A}{\partial T}\right)_V\right\rangle^2\right] - T\left\langle\left(\frac{\partial^2 A}{\partial T^2}\right)_V\right\rangle. \end{aligned} \tag{S36}$$

The first term in the RHS is the fluctuation of the energy field driving the ion dynamics with $T^\mathrm{el} = T$. It is immediate to show that it equals $\lim_{\Delta T\to 0}\frac{1}{\Delta T}[\left\langle A(T^\mathrm{el}=T)\right\rangle_{N,V,T+\Delta T} - \left\langle A(T^\mathrm{el}=T)\right\rangle_{N,V,T}]$, i.e., where $T^\mathrm{el}$ is not changed even if the ionic temperature is varied. The last term at RHS is the average contribution to the heat capacity coming from electronic excitations. The middle terms account for further correlations between the free energy and the electronic entropy, and for the variance of the electronic entropy, respectively. In general, they cannot be neglected.

For the isobaric heat capacity, we follow an analogous derivation, starting with the enthalpy defined from the isothermal-isobaric partition function

$$H \equiv \frac{3}{2}N_\mathrm{i}k_\mathrm{B}T + k_\mathrm{B}T^2\left(\frac{\partial \ln\mathcal{Z}}{\partial\beta}\right)_p, \qquad \text{where} \quad \mathcal{Z} \equiv \sum_V\sum_{\mathbf{R}|_V}\exp\left[-\frac{A(\mathbf{R},\beta)+pV}{k_\mathrm{B}T}\right] \tag{S37}$$

The state of the system is here characterized by a volume $V$ and a given atomic configuration at that volume, $\mathbf{R}|_V$. Therefore,

$$\begin{aligned} H &= \frac{3}{2}N_\mathrm{i}k_\mathrm{B}T + \frac{1}{\mathcal{Z}}\sum_V\sum_{\mathbf{R}|_V}\left[A + pV - T\left(\frac{\partial(A+pV)}{\partial T}\right)_p\right]\exp\left[-\frac{A(\mathbf{R},T)+pV}{k_\mathrm{B}T}\right] \\ &= \frac{1}{\mathcal{Z}}\sum_V\sum_{\mathbf{R}|_V}\left[E(\mathbf{R}|_V,\beta)+pV\right]\exp\left[-\frac{A(\mathbf{R},T)+pV}{k_\mathrm{B}T}\right], \end{aligned} \tag{S38}$$

where we employed

$$\left(\frac{\partial A}{\partial T}\right)_p = \left(\frac{\partial A}{\partial T}\right)_V + \left(\frac{\partial A}{\partial V}\right)_T\left(\frac{\partial V}{\partial T}\right)_p = -S - pV\alpha_p, \qquad \text{and} \quad \left(\frac{\partial pV}{\partial T}\right)_p = +pV\alpha_p, \tag{S39}$$

where $\alpha_p = \frac{1}{V}\left(\frac{\partial V}{\partial T}\right)_p$ is the isobaric expansion coefficient. The isobaric heat capacity can be obtained from finite differences of the enthalpy $H$ in $NpT$ simulations:

$$C_p = \frac{3}{2}N_\mathrm{i}k_\mathrm{B} + \frac{\left\langle E(T^\mathrm{el}=T+\Delta T)\right\rangle_{N,p,T+\Delta T} - \left\langle E(T^\mathrm{el}=T)\right\rangle_{N,p,T}}{\Delta T} + p\frac{\langle V\rangle_{N,p,T+\Delta T} - \langle V\rangle_{N,p,T}}{\Delta T} \tag{S40}$$

In order to check convergence, we performed another simulation of a 1024-atom system at $P = 400$GPa and $T = 20,000$K using the same GAP model used for the other ML simulations at $T^\mathrm{el} = 0$K, and computed the heat capacity from enthalpy fluctuations. We found $C_p(N = 1024) = (2.12 \pm 0.07)k_B$, which in good agreement with $C_p(N = 128) = (1.98 \pm 0.03)k_B$.

## S10. FLUCTUATION FORMULAS IN THE CONTEXT OF $T$-DEPENDENT POTENTIALS

In this Section we provide a derivation of the link between finite-difference and fluctuation formulations of the heat capacity, as in Eq. (S35). In particular, we aim at computing $T$-derivatives of

$$\langle O(T)\rangle = \sum_\nu O_\nu(T)\frac{e^{-W_\nu(T)/k_BT}}{Z(T)}, \qquad Z(T) = \sum_\nu e^{-W_\nu(T)/k_BT} \tag{S41}$$

Therefore:

$$\begin{aligned}\frac{\partial}{\partial T}\langle O(T)\rangle &= \frac{\partial}{\partial T}\sum_\nu O_\nu(T)\frac{e^{-W_\nu(T)/k_BT}}{Z(T)}\\ &= \frac{1}{Z(T)}\sum_\nu\left[\frac{\partial O_\nu(T)}{\partial T}e^{-W_\nu(T)/k_BT} + O_\nu(T)\frac{\partial e^{-W_\nu(T)/k_BT}}{\partial T}\right] - \sum_\nu O_\nu(T)\frac{e^{-W_\nu(T)/k_BT}}{[Z(T)]^2}\frac{\partial}{\partial T}\sum_\mu e^{-W_\mu(T)/k_BT}.\end{aligned} \tag{S42}$$

Since

$$\frac{\partial}{\partial T}e^{-W_\nu(T)/k_BT} = \frac{e^{-W_\nu(T)/k_BT}}{k_BT}\left[\frac{W_\nu(T)}{T} - \frac{\partial W_\nu(T)}{\partial T}\right],$$

we have

$$\begin{aligned}\frac{\partial}{\partial T}\langle O(T)\rangle = &\sum_\nu\left[\frac{\partial O_\nu(T)}{\partial T} + \frac{1}{k_BT}O_\nu(T)\left(\frac{W_\nu(T)}{T} - \frac{\partial W_\nu(T)}{\partial T}\right)\right]\frac{e^{-W_\nu(T)/k_BT}}{Z(T)}\\ &-\sum_\nu O_\nu(T)\frac{e^{-W_\nu(T)/k_BT}}{Z(T)}\sum_\mu\frac{1}{k_BT}\left[\frac{W_\mu(T)}{T} - \frac{\partial W_\mu(T)}{\partial T}\right]\frac{e^{-W_\mu(T)/k_BT}}{Z(T)}\end{aligned} \tag{S43}$$

that is

$$\frac{\partial\langle O\rangle}{\partial T} = \frac{1}{k_BT^2}\left(\langle O\,W\rangle - \langle O\rangle\langle W\rangle\right) - \frac{1}{k_BT}\left(\left\langle O\,\frac{\partial W}{\partial T}\right\rangle - \langle O\rangle\left\langle\frac{\partial W}{\partial T}\right\rangle\right) + \left\langle\frac{\partial O}{\partial T}\right\rangle. \tag{S44}$$

---


[1] I. Lomonosov and V. Gryaznov, Contributions to Plasma Physics **56**, 302 (2016).

[2] R. W. Lee, S. J. Moon, H.-K. Chung, W. Rozmus, H. A. Baldis, G. Gregori, R. C. Cauble, O. L. Landen, J. S. Wark, A. Ng, S. J. Rose, C. L. Lewis, D. Riley, J.-C. Gauthier, and P. Audebert, J. Opt. Soc. Am. B **20**, 770 (2003).

[3] P. Giannozzi, S. Baroni, N. Bonini, M. Calandra, R. Car, C. Cavazzoni, D. Ceresoli, G. L. Chiarotti, M. Cococcioni, I. Dabo, A. Dal Corso, S. de Gironcoli, S. Fabris, G. Fratesi, R. Gebauer, U. Gerstmann, C. Gougoussis, A. Kokalj, M. Lazzeri, L. Martin-Samos, N. Marzari, F. Mauri, R. Mazzarello, S. Paolini, A. Pasquarello, L. Paulatto, C. Sbraccia, S. Scandolo, G. Sclauzero, A. P. Seitsonen, A. Smogunov, P. Umari, and R. M. Wentzcovitch, Journal of physics: Condensed matter **21**, 395502 (2009).

[4] P. Giannozzi, O. Andreussi, T. Brumme, O. Bunau, M. B. Nardelli, M. Calandra, R. Car, C. Cavazzoni, D. Ceresoli, M. Cococcioni, N. Colonna, I. Carnimeo, A. D. Corso, S. de Gironcoli, P. Delugas, R. A. DiStasio, A. Ferretti, A. Floris, G. Fratesi, G. Fugallo, R. Gebauer, U. Gerstmann, F. Giustino, T. Gorni, J. Jia, M. Kawamura, H.-Y. Ko, A. Kokalj, E. Küçükbenli, M. Lazzeri, M. Marsili, N. Marzari, F. Mauri, N. L. Nguyen, H.-V. Nguyen, A. O. de-la Roza, L. Paulatto, S. Poncé, D. Rocca, R. Sabatini, B. Santra, M. Schlipf, A. P. Seitsonen, A. Smogunov, I. Timrov, T. Thonhauser, P. Umari, N. Vast, X. Wu, and S. Baroni, Journal of Physics: Condensed Matter **29**, 465901 (2017).

[5] P. Giannozzi, O. Baseggio, P. Bonfà, D. Brunato, R. Car, I. Carnimeo, C. Cavazzoni, S. de Gironcoli, P. Delugas, F. F. Ruffino, A. Ferretti, N. Marzari, I. Timrov, A. Urru, and S. Baroni, The Journal of Chemical Physics **152**, 154105 (2020).

[6] K. Berland, V. R. Cooper, K. Lee, E. Schröder, T. Thonhauser, P. Hyldgaard, and B. I. Lundqvist, Reports on Progress in Physics **78**, 066501 (2015).

[7] T. Thonhauser, S. Zuluaga, C. Arter, K. Berland, E. Schröder, and P. Hyldgaard, Physical Review Letters **115** (2015), 10.1103/physrevlett.115.136402.

[8] D. C. Langreth, B. I. Lundqvist, S. D. Chakarova-Käck, V. R. Cooper, M. Dion, P. Hyldgaard, A. Kelkkanen, J. Kleis, L. Kong, S. Li, P. G. Moses, E. Murray, A. Puzder, H. Rydberg, E. Schröder, and T. Thonhauser, Journal of Physics: Condensed Matter **21**, 084203 (2009).

[9] T. Thonhauser, V. R. Cooper, S. Li, A. Puzder, P. Hyldgaard, and D. C. Langreth, Physical Review B **76**, 125112 (2007).

[10] M. Schlipf and F. Gygi, Computer Physics Communications **196**, 36 (2015).
[11] N. Marzari, D. Vanderbilt, A. De Vita, and M. C. Payne, Phys. Rev. Lett. **82**, 3296 (1999).
[12] J. P. Perdew, K. Burke, and M. Ernzerhof, Physical Review Letters **77**, 3865 (1996).
[13] A. P. Thompson, H. M. Aktulga, R. Berger, D. S. Bolintineanu, W. M. Brown, P. S. Crozier, P. J. in 't Veld, A. Kohlmeyer, S. G. Moore, T. D. Nguyen, R. Shan, M. J. Stevens, J. Tranchida, C. Trott, and S. J. Plimpton, Comp. Phys. Comm. **271**, 108171 (2022).
[14] A. P. Bartók, R. Kondor, and G. Csányi, Phys. Rev. B **87**, 184115 (2013).
[15] S. De, A. P. Bartók, G. Csányi, and M. Ceriotti, Phys. Chem. Chem. Phys. **18**, 13754 (2016).
[16] M. J. Willatt, F. Musil, and M. Ceriotti, J. Chem. Phys. **150**, 154110 (2019).
[17] F. Musil, M. Veit, A. Goscinski, G. Fraux, M. J. Willatt, M. Stricker, T. Junge, and M. Ceriotti, The Journal of Chemical Physics **154**, 114109 (2021).
[18] C. Ben Mahmoud, A. Anelli, G. Csányi, and M. Ceriotti, Phys. Rev. B **102**, 235130 (2020).
[19] G. Imbalzano, A. Anelli, D. Giofré, S. Klees, J. Behler, and M. Ceriotti, J. Chem. Phys. **148**, 241730 (2018).
